# Supplementary material for: Few-Shot, No Problem: Descriptive Continual Relation Extraction
Source: arXiv:2502.20596 source file (2025-02-27)
Supplement: Supplementary file 1 [file appendix.tex]

\begin{figure*}[ht]
    \centering
    \includegraphics[width=\textwidth]{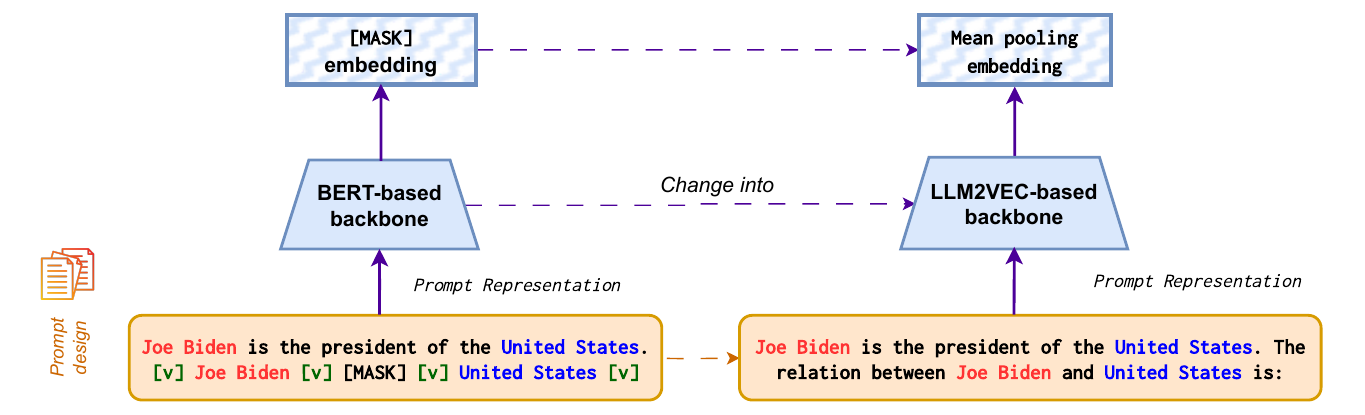}
    \caption{Adapting LLM2Vec for ours architecture}
    \label{fig:change_backbone} 
\end{figure*}

\section{Experimental Details}
\label{appx_implementation}

% Our source code is available at \\ \url{https://anonymous.4open.science/r/DCRE-3BC0}
% \subsubsection{Model architecture}

\subsection{Datasets}
Our experiments utilize the following two benchmarks:
\begin{itemize}
    \item \textbf{FewRel} \cite{han-etal-2018-fewrel} includes 100 relations with 70,000 samples. Following \citet{qin-joty-2022-continual}, we employ a setup with 80 relations, partitioned into 8 tasks, each comprising 10 relations \textit{(10-way)}. Task $\mathcal{T}^1$ includes 100 samples per relation, whereas the remaining tasks are characterized as few-shot tasks conducted under \textit{5-shot} settings.

    \item \textbf{TACRED} \cite{zhang-etal-2017-position} encompasses 42 relations with 106,264 samples extracted from Newswire and Web documents. Consistent with the approach outlined by \citet{qin-joty-2022-continual}, we exclude instances labeled as "no\_relation" and allocate the remaining 41 relations across 8 tasks. Task $\mathcal{T}^1$ comprises 6 relations, each with 100 samples, while each subsequent tasks involve 5 relations \textit{(5-way)} in \textit{5-shot} setups.
    
\end{itemize}

\subsection{Baselines}
\label{sec:appendix_baseline}

In this section, we briefly describe some state-of-the-art methods in FCRE that appear as benchmarking baselines in our evaluations, including:

\begin{itemize}
    \item \textbf{SCKD} \cite{wang-etal-2023-serial} adopts a systematic strategy for knowledge distillation, which aims to preserve old knowledge from previous tasks. Besides, this method employs contrastive learning techniques with pseudo samples to enhance the distinguishability between representations of different relations.

    \item \textbf{CPL} \cite{ma-etal-2024-making} proposes a Contrastive Prompt Learning framework, which designs prompts to generalize across categories and uses margin-based contrastive learning to handle hard samples, thus reducing catastrophic forgetting and overfitting. Besides, the authors employ a memory augmentation strategy to generate diverse samples with ChatGPT, further mitigating overfitting in low-resource scenarios of FCRE.

     \item \textbf{RP-CRE} \cite{cui-etal-2021-refining}: The approach tackles Continual Relation Extraction (CRE) by capitalizing on memorized samples to mitigate the forgetting of previous relations. It employs K-means clustering to identify prototypes that represent each relation based on stored samples. These prototypes are subsequently utilized to refine embeddings of subsequent samples, enabling the model to preserve knowledge of past relations while learning new ones. This methodology enhances memory utilization compared to previous CRE models, resulting in improved performance.

    \item \textbf{CRL} \cite{zhao-etal-2022-consistent}: addresses the issue of catastrophic forgetting by adopting a consistent representation learning strategy. It emphasizes the preservation of stable relation embeddings via contrastive learning and knowledge distillation during the replay of memorized samples. The method involves supervised contrastive learning on a memory bank specific to each new task, followed by contrastive replay of memory samples and knowledge distillation to retain historical relation knowledge. Through this approach, effective alleviation of forgetting is achieved via consistent representation learning.

    \item \textbf{CRECL} \cite{hu-etal-2022-improving}: extends beyond conventional few-shot learning by imposing additional constraints on training data. It accomplishes this by integrating information regarding support instances to augment instance representations. Furthermore, it advocates for open-source task enrichment to facilitate cross-domain knowledge aggregation and introduces the TinyRel-CM dataset tailored specifically for few-shot relation classification with restricted training data. Experimental results illustrate its efficacy in enhancing performance under conditions of limited data availability.

    \item \textbf{ERDA} \cite{qin-joty-2022-continual}: This study introduces Continual Few-Shot Relation Learning (CFRL) as a novel challenge, recognizing the constraints of current methodologies that demand substantial labeled data for new tasks. CFRL endeavors to acquire knowledge of novel relations with minimal data while averting catastrophic forgetting. Addressing this challenge, ERDA presents a methodology grounded in embedding space regularization and data augmentation. This strategy imposes constraints on relational embeddings and integrates supplementary relevant data through self-supervision. Extensive experimentation showcases ERDA's substantial performance enhancements over prior state-of-the-art approaches in CFRL scenarios. 
    
    \item \textbf{ConPL} \cite{DBLP:conf/acl/ChenWS23} introduces a method comprising three core components: a prototype-based classification module, a memory-enhanced module, and a consistent learning module designed to maintain distribution consistency and mitigate forgetting. Furthermore, ConPL employs prompt learning to enhance representation learning and integrates focal loss to reduce confusion among closely related classes.
    \
    \item \textbf{MI} \cite{tran-etal-2024-preserving} introduces a novel framework leveraging often-discarded language model heads to preserve prior knowledge from pre-trained backbones. By employing a mutual information maximization strategy, this method aligns the primary classification head with retained backbone knowledge, enhancing model performance.
\end{itemize}

It is noteworthy that we reproduce the results of ConPL \cite{chen-etal-2023-consistent} under the same settings as SCKD and CPL. This is because the evaluation strategy in the original paper is impractical for continual learning scenarios.

\subsection{Architecture}

\begin{itemize}
    \item For BERT-based models: We use BERT-base-uncased checkpoint\footnote{\url{https://huggingface.co/bert-base-uncased}}  on Hugging Face.
    \item For LLM2Vec-based models: We use the Meta-Llama-3-8B-Instruct-mntp-supervised \footnote{\url{https://huggingface.co/McGill-NLP/LLM2Vec-Meta-Llama-3-8B-Instruct-mntp-supervised}} checkpoint on Hugging Face.
\end{itemize}

% In addition, Figure \ref{fig:change_backbone} depicts the difference in architecture and input design when using the BERT-based backbone and the LLM2Vec-based backbone. In order to exploit LLM2Vec for FCRE problems, we need to apply the current SOTA methods for this type of architecture, which were originally designed for "encoder-only" models (BERT). 

In addition, Figure \ref{fig:change_backbone} depicts the difference in architecture and input design when using the BERT-based backbone and the LLM2Vec-based backbone. Unlike BERT, which uses the "MASK" token during pretraining, the LLM2Vec model does not. As suggested by \citet{llm2vec}, the mean pooling strategy yields the best performance for LLM2Vec. Therefore, we replace the hybrid prompt with a hard prompt and adopt the mean pooling strategy to obtain the input representation.

% Since the LLM2Vec used in our experiment is a 'decoder-only' model with an auto-regressive mechanism \citep{DBLP:journals/corr/abs-1711-09534, DBLP:journals/corr/abs-1906-08237}, we have to modify the designs of BERT ("encoder only" model) to accommodate this architecture.

\subsection{Evaluation Protocol and Training Configurations}
For each reported result, we conduct 6 independent runs with different random seeds and report the mean and the corresponding standard deviation.
\label{appx:eval}
%ConPL compares a model with a predetermined set of candidate classes, while SCKD compares it with all other classes. This paper adopts the SCKD approach as it allows for a more comprehensive evaluation of the model's performance.

\paragraph{Evaluation Metric} 
\begin{itemize}
    \item \textbf{Final average accuracy:} We use final average accuracy to evaluate methods in our experiments. The average accuracy after training task \( T_j \) is calculated as follows:

    \[ ACC_j = \frac{1}{j} \sum_{i=1}^{j} ACC_{j,i} \]

    where \( ACC_{j,i} \) is the accuracy on the test set of task \( T_i \) after training the model on task \( T_j \). 

    \item \textbf{Accuracy drop:} indicates the decrease in average accuracy after training all $T$ tasks on each benchmark.

    \[
    \Delta = ACC_T - ACC_1
    \]
\end{itemize}

\paragraph{Training Configuration}

Details of hyperparameter search:
\begin{itemize}
    \item Learning rate: \{{$\mathbf{1\times 10^{-5}}$}, $2\times 10^{-5}$, $1\times 10^{-4}$\}
    \item $\alpha$: \{\textbf{0.4}, 0.5\}
    \item $\beta_{\textrm{SC}}$: \{0.5, \textbf{1.0}, 1.5, 2.0, 2.5\}
    \item $\beta_{\textrm{MI}}$:   \{0.5, \textbf{1.0}, 1.5, \textbf{2.0}, 2.5\}
    \item $\beta_{\textrm{HM}}$:   \{\textbf{0.5}, \textbf{1.0}, 1.5, 2.0, 2.5\}
    \item $\beta_{\textrm{ST}}$:   \{0.5, \textbf{1.0}, 1.5, 2.0, 2.5\}
\end{itemize}
% \subsection{Training Configurations}

Additionally, Tables \ref{tab:hyperparameters_bert} and \ref{tab:hyperparameters_llm2vec} provide the optimal values of hyperparameters for each model backbone.

\begin{table}[ht]
    \centering
    \begin{tabular}{lc}
        \hline
        Hyperparameter & Value \\
        \hline
        % Random seed & $100$ \\
        % Batch size & $16$ \\
        Current-task training epochs & $10$ \\
        Rehearsal training epochs & $10$ \\
        Learning rate & $1\times 10^{-5}$ \\
        % Optimizer & Adam\\
        $\epsilon$ & 60 \\
        $\alpha$ & 0.4 \\
        \hline
        Encoder output size & $768$ \\
        BERT input max length & $256$ \\
        Margin $m$ for Hard Margin Loss & 0.5 \\ 
        \hline
        $\beta_{\textrm{SC}}$ & $1.0$ \\
        $\beta_{\textrm{MI}}$ (FewRel) & $1.0$ \\
        $\beta_{\textrm{MI}}$ (TACRED) & $2.0$ \\
        
        $\beta_{\textrm{HM}}$ (FewRel) & $1.0$ \\
        $\beta_{\textrm{HM}}$ (TACRED) & $0.5$ \\
        
        $\beta_{\textrm{ST}}$ & $1.0$ \\

        % margin\_m & 0.3 \\
        % normalization\_k & 0.5 \\
        % temperature\_$\tau$ & 0.1 \\
        % contrastive\_sample\_number & 500 \\
        \hline
        Soft prompt initialization & Random \\
        Soft prompt phrase length & 3 \\
        Soft prompt number of phrases & 4 \\
        \hline
        % ChatGPT\_temperature & 0 \\
        % generated\_number\_FewRel & 2 \\
        % generated\_number\_TACRED & 5 \\
        % \hline
    \end{tabular}
    \caption{Hyperparameters for the BERT-backbone setting}
    \label{tab:hyperparameters_bert}
\end{table}

\begin{table}[ht]
    \centering
    \begin{tabular}{lc}
        \hline
        Hyperparameter & Value \\
        \hline
        % Random seed & 100 \\
        % Batch size & 2 \\
        Encoder output size & $4096$ \\
        Current-task training epochs & 10 \\
        Rehearsal training epochs & 10 \\
        Learning rate & $1\times 10^{-5}$ \\
        % Optimizer & Adam \\
        $\epsilon$ & 60 \\
        $\alpha$ & 0.4 \\
        Margin $m$ for Hard Margin Loss & 0.5 \\
        \hline
        % Target modules & q\_proj,
        %         v\_proj,
        %         k\_proj,
        %         o\_proj,
        %         gate\_proj,
        %         up\_proj,
        %         down\_projrelation\_description\_detail
        % \\
        Lora alpha & 16 \\
        Lora rank & 8 \\
        Lora dropout & 0.05 \\
        \hline
        $\beta_{\text{SC}}$ & 1.0 \\
        $\beta_{\text{MI}}$ (FewRel) & 1.0 \\
        $\beta_{\text{MI}}$ (TACRED) & 2.0 \\
        
        $\beta_{\text{HM}}$ (FewRel) & 1.0 \\
        $\beta_{\text{HM}}$ (TACRED) & 0.5 \\
        
        $\beta_{{\text{ST}}}$ & 1.0 \\
        \hline
        % margin\_m & 0.3 \\
        % normalization\_k & 0.5 \\
        % temperature\_$\tau$ & 0.1 \\
        % contrastive\_sample\_number & 500 \\
        % \hline
        % Prompt initialization & Hard prompt \\
        % soft\_prompt\_length & 3 \\
        % soft\_prompt\_number & 4 \\
        % \hline
        % ChatGPT\_temperature & 0 \\
        % generated\_number\_FewRel & 2 \\
        % generated\_number\_TACRED & 5 \\
        % \hline
    \end{tabular}
    \caption{Hyperparameters setting with LLM2vec backbone.}
    \label{tab:hyperparameters_llm2vec}
\end{table}

\subsection{Prompt Template}
\label{apdx:prompt_template}

Table \ref{tab:judge_prompt_stability} illustrates a prompt used to generate label descriptions for a relation called {\textit{"place served by transport hub"}} and its respective output, during training in our strategy.

\section{Additional experimental results}

\subsection{Effect of the number of generated descriptions for each relation}

Table \ref{tab:k} reports the final accuracy of BERT-based models on two benchmarks when varying the number of generated descriptions $K$. The results show that using multiple generated descriptions is better than using just one, as many generated samples help provide more specific, diverse, and semantically rich information, thereby making representation learning more comprehensive and effective. However, if $K$ is too large, our observations indicate that LLMs like Gemini can generate biased and low-quality samples, which negatively affect model performance. In particular, the best accuracy is achieved when $K=3$ on FewRel and $K=7$ on TACRED.

% The result of $K=7$ on FewRel is worse than $K=1$ is an exception. This might be because  

\begin{table}[ht]
    \centering
    % \resizebox{0.45\textwidth}{!}{
    \setlength{\tabcolsep}{1mm}
    \begin{tabular}{lcc}
    \hline 
    Num of generated descritions & \multicolumn{1}{c}{FewRel} & \multicolumn{1}{c}{TACRED}\\
    % \cmidrule(lr){2-3} \cmidrule(lr){4-5} 
    % & BERT & LLM2Vec & BERT & LLM2Vec  \\
    \hline \hline \\
    K = 1  & 68.24 & 63.21 \\ 
    K = 3 & \textbf{69.42} & 64.92\\
    K = 5 & \underline{69.14} & 65.45 \\ 
    K = 7 & 68.92 & \textbf{67.85} \\
    K = 10  & 68.94 & \underline{67.29} \\ 
    
    \hline
    \end{tabular}%}
    \caption{Final accuracy (\%) after 8 tasks, when varying the number of generated desciptions}
    \label{tab:k}
\end{table}

Moreover, we provide an ablation study demonstrating the importance of each component in the objective function when using the optimal value of $K$. The results depict that on both datasets, $\mathcal{L}_{MI}$, designed to maximize the mutual information between the input samples' hidden representations and their corresponding retrieved descriptions, plays the most vital role. Its absence can cause the model to lose 4-5\% in final accuracy.

\begin{table}[ht]
    \centering
    % \resizebox{0.45\textwidth}{!}{
    \setlength{\tabcolsep}{1mm}
    \begin{tabular}{lcccc}
    \hline 
    \multirow{2}{*}{Method} & \multicolumn{2}{c}{BERT}\\
    \cmidrule(lr){2-3}
    & FewRel $(K = 3)$ & TACRED $(K = 7)$ \\
    \hline \hline \\
    \text{DCRE (Our)} & \textbf{69.42} & \textbf{67.85} &\\
    % \text{DCRE (Our)} & 67.82 & 64.92 \\
    \quad  \small \text{w/o $\mathcal{L}_{\textrm{SC}}$} & {67.12} &  \underline{67.11} & \\
    \quad  \small \text{w/o $\mathcal{L}_{\textrm{MI}}$} & 65.96 & 62.41  \\
    \quad  \small \text{w/o $\mathcal{L}_{\textrm{HM}}$} & \underline{69.35} & {66.46}\\
    \quad  \small \text{w/o $\mathcal{L}_{\textrm{ST}}$} & 69.03 & 66.12 & \\
    \hline
    \end{tabular}%}
        \caption{Ablation study with optimal values of $K$.}
    \label{tab:ablation_study}
\end{table}

\begin{figure*}[t]
    \centering
    \includegraphics[width=0.75\textwidth]{imgs/bert_predict.pdf}
    \caption{NCM and DRI prediction, BERT-based models}
    \label{fig:bert_prediction} 
\end{figure*}

\subsection{NCM and DRI prediction}

Figures \ref{fig:bert_prediction} and \ref{fig:llm_prediction} compare model performance when using the conventional prediction method (NCM), and our proposed prediction strategy, DRI. The results show that, in most cases, our DRI outperforms NCM. In particular, on FewRel, DRI improves final accuracy by 1-2\% compared to NCM. Notably, on the TACRED, this gap can be achieved by 4-5\%.

\begin{figure*}[ht]
    \centering
    \includegraphics[width=0.75\textwidth]{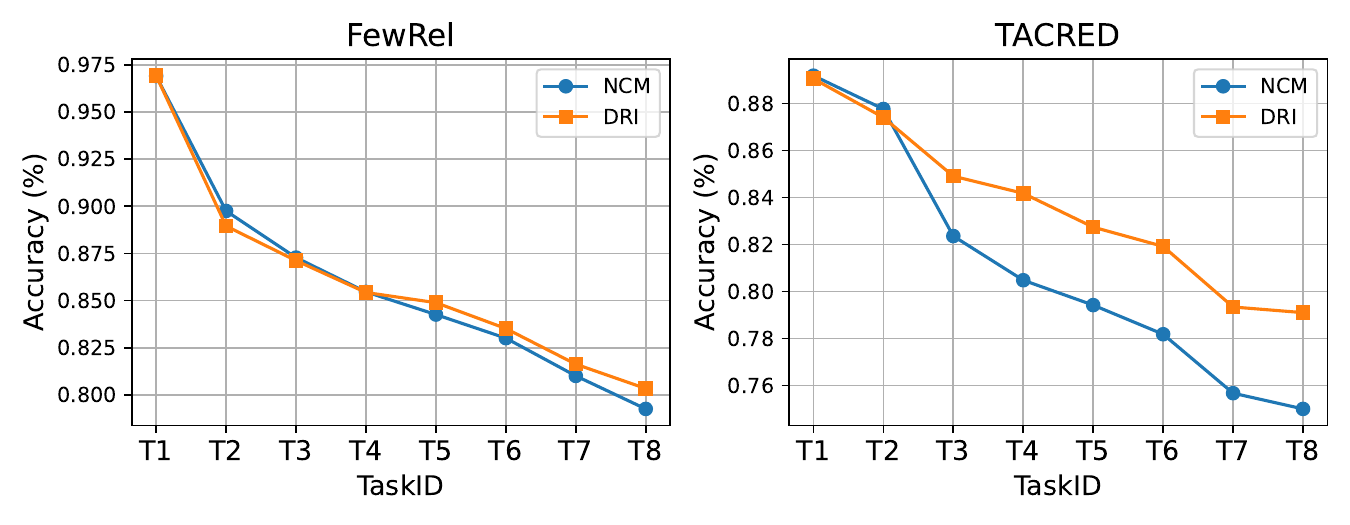}
    \caption{NCM and DRI prediction, LLM2Vec-based models}
    \label{fig:llm_prediction} 
\end{figure*}

% \begin{figure*}[t]
%     \centering
%     \includegraphics[width=0.3\textwidth]{imgs/tacred-ncm-dri.pdf}
%     \caption{Compare NCM-DRI on Tacred dataset - LLM2vec backbone}
%     \label{fig:change_backbone} 
% \end{figure*}

% \begin{figure*}[t]
%     \centering
%     \includegraphics[width=0.3\textwidth]{imgs/tacred-bert-ncm-dri.pdf}
%     \caption{Compare NCM-DRI on Fewrel dataset - Bert backbone}
%     \label{fig:change_backbone} 
% \end{figure*}

% \begin{figure*}[t]
%     \centering
%     \includegraphics[width=0.3\textwidth]{imgs/fewrel-bert-ncm-dri.pdf}
%     \caption{Compare NCM-DRI on Tacred dataset - Bert backbone}
%     \label{fig:change_backbone} 
% \end{figure*}

\begin{table*}[ht]
    % \scriptsize
    % \texttt
    \centering
\begin{tabular}{@{}p{\linewidth}@{}}
% \hline
\textbf{Prompt for generate label description} \\
\hline
You are a professional data scientist, working in a relation extraction project. \\
Given a relation and its description, you are asked to write a more detailed description of the relation and provide 3 sentence examples of the relation. \\
The relation is: place served by transport hub \\
The description is: territorial entity or entities served by this transport hub (airport, train station, etc.) \\
Please generate \textbf{2} diverse samples of (relation description, examples). \\
Your response: \\
\hline \\

\textbf{Output:} \\
\hline
% This relation identifies the geographical region or regions that a specific transportation hub, such as an airport, train station, bus terminal, or port, primarily serves. It defines the area from which the hub draws passengers or goods and the area to which it connects them.\\
% Examples: \\
% London Gatwick Airport serves the city of London and its surrounding areas.\\
% Union Station in Chicago serves as a hub for the Midwest region, connecting passengers to various destinations.\\
% The Port of Rotterdam, located in the Netherlands, serves as a major transportation hub for goods entering and leaving Europe.\\
This relation identifies the geographic areas or communities that are directly connected to and supported by a specific transport hub, such as an airport, train station, or bus terminal, emphasizing the role of the hub in providing access to transportation services for these areas.\\
Examples: \\
- Heathrow Airport serves the Greater London area, providing access to travelers from London and surrounding towns. \\
- Union Station in Washington, D.C. serves the metropolitan area, facilitating travel for residents and visitors in Maryland and Virginia. \\
- Los Angeles International Airport (LAX) serves not only Los Angeles but also the wider Southern California region, including cities like Santa Monica and Long Beach.\\
\hline 
This relation captures the locations or regions that benefit from the operational capabilities of a transport hub, highlighting its significance in regional connectivity and economic activity.\\
Examples: \\
- Chicago O'Hare International Airport serves the entire Chicago metropolitan area, enhancing accessibility for surrounding suburbs.\\
- Penn Station in New York City is a critical transport hub that serves travelers from New Jersey, New York, and Connecticut.\\
- Dallas/Fort Worth International Airport serves the Dallas and Fort Worth areas, acting as a key transit point for the entire North Texas region.\\
% \hline 
% This relation entails the specific towns, cities, or regions that are facilitated by a transport hub, underlining the importance of the hub for local and regional transportation links.\\
% Examples: \\
% - San Francisco International Airport serves not just San Francisco but also neighboring counties like San Mateo and Marin., \\
% - The Eurostar terminal at St. Pancras International serves London and connects to various regions in France and Belgium., \\
% - Vancouver International Airport (YVR) serves the city of Vancouver as well as the surrounding areas of British Columbia, including Richmond and Burnaby.	\\
\hline
% \bottomrule
\end{tabular}
    \caption{Example generated label description}
    \label{tab:judge_prompt_stability}
\end{table*}
